# Supplementary material for: StateRAG: Typed State Contracts for Complex Retrieval-Augmented Generation
Source: arXiv:2605.25379 source file (2026-11-10)
Supplement: Supplementary file 1 [file appendix.tex]

\documentclass[letterpaper]{article} % DO NOT CHANGE THIS
\usepackage[preprint]{aaai2027}  % DO NOT CHANGE THIS
% The serif, sans-serif, and monospaced fonts are loaded automatically by
% aaai2027.sty (newtxtext, helvet, courier). DO NOT add \usepackage{times},
% \usepackage{helvet}, \usepackage{courier}, or any other font package.
\usepackage[hyphens]{url}  % DO NOT CHANGE THIS
\usepackage{graphicx} % DO NOT CHANGE THIS
\urlstyle{rm} % DO NOT CHANGE THIS
  % DO NOT CHANGE THIS
\usepackage{natbib}  % DO NOT CHANGE THIS AND DO NOT ADD ANY OPTIONS TO IT
\usepackage{caption} % DO NOT CHANGE THIS AND DO NOT ADD ANY OPTIONS TO IT
\frenchspacing  % DO NOT CHANGE THIS

\usepackage{amsmath}
\usepackage{algorithm}
\usepackage{algpseudocode}

%
% These are recommended to typeset listings but not required. See the subsubsection on listing. Remove this block if you don't have listings in your paper.
\usepackage{newfloat}
\usepackage{listings}
\DeclareCaptionStyle{ruled}{labelfont=normalfont,labelsep=colon,strut=off} % DO NOT CHANGE THIS
\lstset{%
	basicstyle={\footnotesize\ttfamily},% footnotesize acceptable for monospace
	numbers=left,numberstyle=\footnotesize,xleftmargin=2em,% show line numbers, remove this entire line if you don't want the numbers.
	aboveskip=0pt,belowskip=0pt,%
	showstringspaces=false,tabsize=2,breaklines=true}
\floatstyle{ruled}
\newfloat{listing}{tb}{lst}{}
\floatname{listing}{Listing}

%
% Recommended for better-looking tables
\usepackage{booktabs}

%
% Keep the \pdfinfo as shown here. There's no need
% for you to add the /Title and /Author tags.
\pdfinfo{
/TemplateVersion (2027.1)
}

\setcounter{secnumdepth}{2}

% The file aaai2027.sty is the style file for AAAI Press
% proceedings, working notes, and technical reports.
%

% Title

% Your title must be in mixed case, not sentence case.
% That means all verbs (including short verbs like be, is, using,and go),
% nouns, adverbs, adjectives should be capitalized, including both words in hyphenated terms, while
% articles, conjunctions, and prepositions are lower case unless they
% directly follow a colon or long dash
\title{\textsc{StateRAG}: Appendix \& Supplementary Material}
\author{
  Miaohe Niu\textsuperscript{\rm 1},
  Pengxiang Li\textsuperscript{\rm 2}\corresponding,
  Jingbo Zhu\textsuperscript{\rm 1,\rm 3},
  Tong Xiao\textsuperscript{\rm 1,\rm 3}\corresponding
}
\affiliations{
  \textsuperscript{\rm 1}School of Computer Science and Engineering, Northeastern University, China \\
  \textsuperscript{\rm 2}Hong Kong Polytechnic University, China \\
  \textsuperscript{\rm 3}NiuTrans Research, Shenyang, China \\
  niumiaohe@mails.neu.edu.cn,
  pengxiang.li@connect.polyu.hk,
  xiaotong@mail.neu.edu.cn
}

\begin{document}

\maketitle

\section{TAM Construction and Navigation}
\label{sec:supp_tam}

Typed Abstraction Memory (TAM) organizes the source collection associated
with each query as the rooted, typed directed acyclic graph defined in the
main paper. Construction proceeds from Evidence nodes grounded in the source to Relation abstractions and then to Topic abstractions. The
Navigator subsequently traverses this graph under type, width, depth, and
candidate constraints.

\paragraph{Evidence regions.}
Documents are segmented with the retrieval pipeline tokenizer into regions of
384 tokens, with an overlap of 64 tokens between adjacent regions. Each region
retains its source identifier and offsets so that retrieved evidence can be
traced to the original document. The regions are encoded with
\texttt{BAAI/bge-base-en-v1.5} and instantiated as Evidence nodes. For an
Evidence node \(v\), the map \(\rho(v)\) returns its associated retrieval
region.

\paragraph{Typed abstraction construction.}
TAM first applies agglomerative cosine grouping to the Evidence nodes.
Relation groups use a similarity threshold of \(0.78\) and contain at most
eight Evidence nodes. The resulting Relation nodes are grouped into Topic
nodes with a threshold of \(0.70\) and a maximum group size of six Relation
nodes. A node may be assigned to at most two compatible parent groups. This
overlapping assignment permits multiple parent paths while preserving the
acyclic ordering from Root through Topic and Relation to Evidence.

Qwen2.5-7B generates the textual representation \(a(v)\) of each Relation and
Topic node with temperature \(0\). A unique Root node is connected to the
Topic nodes. One TAM is constructed for each query associated source
collection before traversal.

\begin{table*}[t]
\centering
\small
\setlength{\tabcolsep}{7pt}
\begin{tabular}{p{0.27\textwidth}p{0.65\textwidth}}
\toprule
Item & Setting \\
\midrule
Evidence regions &
384 tokenizer tokens with an overlap of 64 tokens \\

Embedding encoder &
\texttt{BAAI/bge-base-en-v1.5} \\

Relation grouping &
Agglomerative cosine grouping with threshold \(0.78\) and at most eight
Evidence nodes per group \\

Topic grouping &
Agglomerative cosine grouping with threshold \(0.70\) and at most six
Relation nodes per group \\

Parent assignment &
At most two compatible parents per node \\

Abstraction generator &
Qwen2.5-7B with temperature \(0\) \\

Trace scorer \(g\) &
Batched Qwen2.5-7B path scoring with temperature \(0\) \\

Navigation limits &
Local branch cap \(B=2\), global beam width \(K=4\), candidate budget
\(C_{\max}=32\) per traversal, and maximum depth \(h_{\max}=3\) \\

Tie breaking &
Stable node order \\

Construction scope &
One TAM for each query associated source collection before traversal \\
\bottomrule
\end{tabular}
\caption{TAM construction and navigation settings.}
\label{tab:supp_tam_settings}
\end{table*}

Algorithm~\ref{alg:supp_tam_construction} summarizes construction. The
grouping operation admits overlapping assignments while enforcing the
similarity, group size, and parent limits in
Table~\ref{tab:supp_tam_settings}.

\begin{algorithm}[!t]
\caption{TAM construction}
\label{alg:supp_tam_construction}
\begin{algorithmic}[1]
\Require Source collection \(\mathcal D\), embedding encoder
\(f_{\mathrm{emb}}\), abstraction generator \(F_a\)
\Ensure Typed graph
\(\mathcal H=
\langle V,E_{\mathcal H},v_{\mathrm{root}},\lambda,a,\rho\rangle\)

\State
\(\mathcal R \gets
\Call{Segment}{\mathcal D,384,64}\)

\State Create one Evidence node \(v_r\) for each \(r\in\mathcal R\)
\State Set
\(\lambda(v_r)=\textsc{Evidence}\),
\(a(v_r)=\operatorname{text}(r)\), and
\(\rho(v_r)=r\)

\State
\(\mathcal G_{\mathrm R}\gets
\Call{CosineGroups}{V_{\mathrm E},f_{\mathrm{emb}},0.78,8,2}\)

\ForAll{\(G\in\mathcal G_{\mathrm R}\)}
    \State Create a Relation node \(v_G\)
    \State Set
    \(\lambda(v_G)=\textsc{Relation}\) and
    \(a(v_G)=F_a(G)\)
    \State Add an edge from \(v_G\) to every node in \(G\)
\EndFor

\State
\(\mathcal G_{\mathrm T}\gets
\Call{CosineGroups}{V_{\mathrm R},f_{\mathrm{emb}},0.70,6,2}\)

\ForAll{\(G\in\mathcal G_{\mathrm T}\)}
    \State Create a Topic node \(v_G\)
    \State Set
    \(\lambda(v_G)=\textsc{Topic}\) and
    \(a(v_G)=F_a(G)\)
    \State Add an edge from \(v_G\) to every node in \(G\)
\EndFor

\State Create the unique Root node \(v_{\mathrm{root}}\)
\State Set
\(\lambda(v_{\mathrm{root}})=\textsc{Root}\)
\State Add an edge from \(v_{\mathrm{root}}\) to every Topic node
\State \Return \(\mathcal H\)
\end{algorithmic}
\end{algorithm}

\paragraph{Typed navigation.}
For a query \(q\) and committed plan \(p_q^{t+1}\), the Navigator begins at
\(v_{\mathrm{root}}\). Candidate extensions are first filtered by the
admissible type transition set \(\mathcal A\). Type filtering therefore occurs
before path scoring.

The scorer evaluates a trace \(\pi\) using

\begin{equation}
G_q^{t+1}(\pi)
=
g\!\left(
q,
p_q^{t+1},
a\!\left(\operatorname{last}(\pi)\right)
\right).
\label{eq:supp_trace_score}
\end{equation}

The implementation uses batched Qwen2.5-7B scoring with temperature \(0\).
For each active trace, at most two admissible child extensions are retained.
The global beam then keeps at most four incomplete traces. A traversal
evaluates at most 32 candidate extensions and performs at most three graph
expansions. Equal scores are resolved by stable node order.

Completed traces ending at Evidence nodes are stored separately from the
active beam. Navigation terminates when the beam is empty, the candidate
budget is exhausted, or the depth limit is reached.

\begin{algorithm}[!htbp]
\caption{Typed TAM navigation}
\label{alg:supp_tam_navigation}
\begin{algorithmic}[1]
\Require Query \(q\), committed plan \(p_q^{t+1}\), TAM \(\mathcal H\),
transition set \(\mathcal A\), scorer \(g\)
\Ensure Path proposal \(\widehat{\pi}_q^{t+1}\) or failure \(\bot\)

\State
\(\mathcal B_0\gets
\{\langle v_{\mathrm{root}}\rangle\}\)

\State
\(\mathcal Q\gets\emptyset\),
\(c\gets0\)

\For{\(\ell=0,\ldots,2\)}
    \State \(\mathcal X\gets\emptyset\)

    \ForAll{\(\pi\in\mathcal B_\ell\)}
        \If{\(\lambda(\operatorname{last}(\pi))
        =\textsc{Evidence}\)}
            \State \(\mathcal Q\gets\mathcal Q\cup\{\pi\}\)
        \Else
            \State Generate extensions whose type pairs belong to
            \(\mathcal A\)
            \State Add admissible extensions to \(\mathcal X\)
        \EndIf
    \EndFor

    \If{\(\mathcal X=\emptyset\) or \(c\geq32\)}
    \State \textbf{break}
\EndIf

\State
\(\mathcal X\gets
\Call{SelectBudget}{\mathcal X,32-c}\)

\If{\(\mathcal X=\emptyset\)}
    \State \textbf{break}
\EndIf
    \State Score retained extensions using
    Equation~\ref{eq:supp_trace_score}
    \State Keep at most two extensions for each parent trace
    \State \(c\gets c+|\mathcal X|\)

    \State Add completed extensions in \(\mathcal X\) to \(\mathcal Q\)
    \State
    \(\mathcal B_{\ell+1}\gets\)
    the four highest scoring incomplete extensions in \(\mathcal X\)

    \If{\(\mathcal B_{\ell+1}=\emptyset\)}
        \State \textbf{break}
    \EndIf
\EndFor

\State
\(\mathcal Q_L\gets\mathcal Q\)

\If{\(\mathcal Q_L=\emptyset\)}
    \State \Return \(\bot\)
\EndIf

\State
\(\widehat{\pi}_q^{t+1}
\gets
\operatorname*{arg\,max}_{\pi\in\mathcal Q_L}
G_q^{t+1}(\pi)\)

\State \Return \(\widehat{\pi}_q^{t+1}\)
\end{algorithmic}
\end{algorithm}

The controller validates the returned proposal against
\(\Pi_{\mathcal H}\). After commitment, the terminal Evidence node determines

\begin{equation}
R_q^{t+1}
=
\rho\!\left(
\operatorname{last}
\left(
\pi_q^{t+1}
\right)
\right).
\label{eq:supp_selected_region}
\end{equation}

The Retriever receives only \(R_q^{t+1}\) when constructing its evidence
proposal. If \(\mathcal Q_L\) is empty, the Navigator returns a traversal
failure. Supplementary Section~\ref{sec:supp_lifecycle} specifies how this
required update failure terminates the query without reader admission. TAM
also exposes its leaf count to the compact evidence check defined in that
section.
\FloatBarrier
\section{Lifecycle, Validation, and Persistence Protocol}
\label{sec:supp_lifecycle}

This section specifies the execution protocol that connects typed navigation,
field validation, controller actions, artifact persistence, and final reader
admission. The protocol operates on the query state defined in the main paper
and invokes the final reader only after a terminal action.

\subsection{Initialization and Bypass}
\label{sec:supp_initialization}

For query \(q\), initialization creates \(s_q^0\), obtains the initial candidate
evidence \(E_q^0\), and resolves the artifact identifiers available through
\(U_q^0\). The controller then evaluates the configured compact-evidence
predicate

\begin{equation}
b_q
=
C_{\mathrm{bp}}
\left(
q,
s_q^0,
E_q^0,
\mu_{\mathcal H}
\right)
\in
\{0,1\},
\label{eq:supp_bypass_predicate}
\end{equation}

where \(\mu_{\mathcal H}\) includes the Evidence-leaf count available before
typed navigation. The predicate returns one when the initial evidence is
nonempty, the associated TAM evidence space contains at most five Evidence
leaves, and the selected evidence fits within the reader evidence budget. It is evaluated once before the first MARS cycle.

When \(b_q=1\), the controller selects \(E_{q,\mathrm{bp}}\) from \(E_q^0\)
while preserving the initial retrieval order and provenance. It then enters
\textsc{Bypass}. This branch does not invoke the Navigator and does not commit
a traversal path. When \(b_q=0\), the query enters the ordered role update
cycle.

The Retriever reranks at most 10 Evidence candidates. The initial retrieval
pass retains at most five evidence items, while a revised state retains at
most seven. We set \(T_{\max}=2\), allowing one initial cycle and at most one
revision.
\subsection{Ordered Updates and Validation}
\label{sec:supp_validation}

For a non-bypass query, cycle \(t+1\) begins from the committed state \(s_q^t\).
The controller creates the initial staged state

\begin{equation}
s_q^{t,0}
=
s_q^t
\left[
z
\leftarrow
\left\langle
\textsc{Pending},
\epsilon_{\Delta}
\right\rangle
\right],
\label{eq:supp_staged_initialization}
\end{equation}

where \(\epsilon_{\Delta}\) is the empty justification. The Planner,
Navigator, Retriever, and Verifier execute in this order. They are paired with

\begin{equation}
(f_1,f_2,f_3,f_4)
=
(p,\pi,E,z).
\label{eq:supp_role_fields}
\end{equation}

At stage \(i\), the corresponding role reads the latest staged state and
proposes \(\widehat v_{q,i}^{t+1}\). The field validator computes

\begin{equation}
\alpha_{q,i}^{t+1}
=
V_{f_i}
\left(
\widehat v_{q,i}^{t+1},
s_q^{t,i-1}
\right)
\in
\{0,1\}.
\label{eq:supp_validation_result}
\end{equation}

An accepted proposal is written to its designated field:

\begin{equation}
s_q^{t,i}
=
s_q^{t,i-1}
\left[
f_i
\leftarrow
\widehat v_{q,i}^{t+1}
\right]
\quad
\text{when }
\alpha_{q,i}^{t+1}=1.
\label{eq:supp_validated_update}
\end{equation}

Table~\ref{tab:supp_role_checks} summarizes the four validation checks.

\begin{table}[t]
\centering
\small
\setlength{\tabcolsep}{4pt}
\begin{tabular}{llll}
\toprule
Role & Proposal & Field & Validation \\
\midrule
Planner &
\(\widehat p_q^{t+1}\) &
\(p\) &
Plan schema \\

Navigator &
\(\widehat\pi_q^{t+1}\) &
\(\pi\) &
Typed path \\

Retriever &
\(\widehat E_q^{t+1}\) &
\(E\) &
Provenance \\

Verifier &
\(\widehat z_q^{t+1}\) &
\(z\) &
Verdict record \\
\bottomrule
\end{tabular}
\caption{Role proposals and validation checks.}
\label{tab:supp_role_checks}
\end{table}

The plan check requires a nonempty retrieval objective in the configured plan
schema. The path check requires a completed trace in
\(\Pi_{\mathcal H}\). The evidence check requires every evidence record to
carry valid provenance from the retrieval region associated with the committed
path. The verdict check requires

\begin{equation}
\widehat z_q^{t+1}
=
\left\langle
\widehat\nu_q^{t+1},
\widehat\delta_q^{t+1}
\right\rangle
\in
\mathcal Z
\label{eq:supp_verdict_proposal}
\end{equation}

with
\(\widehat\nu_q^{t+1}\in
\{\textsc{Pass},\textsc{Fail}\}\).
A \textsc{Fail} verdict includes a revision justification
\(\widehat\delta_q^{t+1}\).

A cycle commits only when all four required proposals pass their validation
checks. If a required proposal fails, the preceding staged state is retained
and no next-cycle state is formed. The execution returns \(\bot\), is recorded
as incomplete, and does not enter the final reader. An empty completed-path
set from the Navigator follows the same failure branch.

After all four stages have completed, the controller commits

\begin{equation}
s_q^{t+1}
=
s_q^{t,4}.
\label{eq:supp_cycle_commit}
\end{equation}

The committed verdict is
\(z_q^{t+1}=
\langle
\nu_q^{t+1},
\delta_q^{t+1}
\rangle\).
No evidence update occurs between this commitment and controller action
selection.

\subsection{Controller Actions and Reader Admission}
\label{sec:supp_reader_admission}

For a completed MARS cycle, the controller combines the committed verdict
with the remaining cycle budget:

\begin{equation}
d_q^{t+1}
=
\begin{cases}
\textsc{Release},
&
\nu_q^{t+1}=\textsc{Pass},
\\
\textsc{Revise},
&
\nu_q^{t+1}=\textsc{Fail}
\land
t+1<T_{\max},
\\
\textsc{Fallback},
&
\nu_q^{t+1}=\textsc{Fail}
\land
t+1=T_{\max}.
\end{cases}
\label{eq:supp_controller_action}
\end{equation}

Under \textsc{Revise}, the Verifier justification
\(\delta_q^{t+1}\) is supplied to the Planner as revision context for the next
cycle. The artifact identifiers in \(U\) are refreshed before that cycle
begins. \textsc{Release} and \textsc{Fallback} terminate retrieval.

Fallback evidence is formed from the committed evidence sets produced by the
completed cycles. The merge processes cycles in execution order and preserves
the Retriever ranking within each cycle. Evidence records with the same
identifier are retained once. Records are appended until the reader evidence
budget is reached. If the final record exceeds the remaining budget, its text
is truncated while its identifier and provenance are retained. We denote this
operation by

\begin{equation}
E_{q,\mathrm{fb}}
=
\operatorname{Merge}_{B}
\left(
E_q^1,
\ldots,
E_q^{T_{\max}}
\right),
\label{eq:supp_fallback_merge}
\end{equation}

where \(B\) is the reader evidence budget.

The evidence admitted to the common reader is

\begin{equation}
E_q^\star
=
\begin{cases}
E_{q,\mathrm{bp}},
&
d_q^\star=\textsc{Bypass},
\\
E_q^{t+1},
&
d_q^{t+1}=\textsc{Release},
\\
E_{q,\mathrm{fb}},
&
d_q^{t+1}=\textsc{Fallback}.
\end{cases}
\label{eq:supp_terminal_evidence}
\end{equation}

The common reader entry computes

\begin{equation}
y_q
=
G_{\phi}
\left(
q,
E_q^\star
\right).
\label{eq:supp_reader}
\end{equation}

A query enters this reader only after
\textsc{Bypass}, \textsc{Release}, or \textsc{Fallback}. It does not enter the
reader after \textsc{Revise}, during a staged update, or after a required
update failure. Each query invokes the final reader at most once.

\subsection{Scoped Artifact Persistence}
\label{sec:supp_persistence}

Let
\(\mathcal R_{\mathrm{op}}=\{\mathrm P,\mathrm N,\mathrm R,\mathrm V\}\)
denote the Planner, Navigator, Retriever, and Verifier. Shared Memory Pool (SMP) retains reusable artifact payloads outside the live
query state. For query \(q\), it maintains

\begin{equation}
\mathcal M_q
=
\left(
M_g[\chi_q],
M_t^q,
\left\{
M_a^{q,r}
\right\}_{r\in\mathcal R_{\mathrm{op}}}
\right),
\label{eq:supp_memory_stores}
\end{equation}

where \(M_g[\chi_q]\) is the global store for workload scope \(\chi_q\),
\(M_t^q\) contains artifacts scoped to query \(q\), and \(M_a^{q,r}\)
contains artifacts private to role \(r\). The live field
\(U_q^t\) stores the identifiers of artifacts available to the current cycle.
Their payloads remain in SMP.

Each artifact records its identifier, payload, producer, scope, and source
provenance. SMP admits an operation when the requesting role, operation,
scope, query, and ownership conditions match. Repeated artifacts with the
same identifier are stored once.

Artifacts produced during a cycle remain transient until action selection.
After the action is selected, SMP persists eligible payloads according to
their declared scope. An eligible payload is nonempty, has valid provenance,
and is produced by a role permitted to write to the selected scope. Reference
answers, evaluation labels, and final reader outputs are never eligible for
persistence.

Following \textsc{Revise}, SMP resolves the identifiers available to the next
cycle and refreshes \(U\). Following a terminal action, evidence selection
occurs before persistence. Terminal persistence therefore does not change
\(E_q^\star\).

In the main evaluation, \(M_g\) is initialized at the beginning of each
workload and remains available across its fixed query order.
\(M_t^q\) and the role private stores are cleared when query
execution ends. Artifacts are not transferred across workloads. In the
matched carrier control, both carrier variants additionally clear \(M_g\) at
each query boundary while retaining the remaining SMP behavior.

\subsection{Complete Execution Protocol}
\label{sec:supp_complete_protocol}

Algorithm~\ref{alg:supp_staterag} summarizes the complete protocol. The
operators \(\mathcal O_1,\ldots,\mathcal O_4\) denote the Planner, Navigator,
Retriever, and Verifier. Their designated fields are
\(p,\pi,E,z\).

\begin{algorithm}[!t]
\caption{Complete StateRAG execution protocol.}
\label{alg:supp_staterag}
\small
\begin{algorithmic}[1]
\Require Query \(q\), typed graph \(\mathcal H\), memory pool
\(\mathcal M\), cycle budget \(T_{\max}\), reader evidence budget \(B\)
\Ensure Answer \(y_q\) or incomplete result \(\bot\)

\State
\((s_q^0,E_q^0)
\gets
\operatorname{Initialize}(q,\mathcal H)\)

\State
\(U_q^0
\gets
\operatorname{Resolve}(\mathcal M,q)\)
\State
\(s_q^0
\gets
s_q^0[U\leftarrow U_q^0]\)
\State
\(\mathcal E_{\mathrm{hist}}
\gets
\langle\rangle\)

\State
\(c_q
\gets
\epsilon_{\Delta}\)

\State
\(b_q
\gets
C_{\mathrm{bp}}
(q,s_q^0,E_q^0,\mu_{\mathcal H})\)

\If{\(b_q=1\)}
    \State
    \(d_q^\star
    \gets
    \textsc{Bypass}\)

    \State
    \(E_q^\star
    \gets
    \operatorname{SelectBudget}
    (E_q^0,B)\)
\Else
    \For{\(t=0,\ldots,T_{\max}-1\)}
        \State
        \(s_q^{t,0}
        \gets
        s_q^t
        [
        z
        \leftarrow
        \langle
        \textsc{Pending},
        \epsilon_{\Delta}
        \rangle
        ]\)

        \For{\(i=1,\ldots,4\)}
            \State
            \(\widehat v_{q,i}^{t+1}
            \gets
            \mathcal O_i
            (q,s_q^{t,i-1},c_q,\mathcal H)\)

            \State
            \(\alpha_{q,i}^{t+1}
            \gets
            V_{f_i}
            (
            \widehat v_{q,i}^{t+1},
            s_q^{t,i-1}
            )\)

            \If{\(\alpha_{q,i}^{t+1}=0\)}
                \State
                \Return \(\bot\)
            \EndIf

            \State
            \(s_q^{t,i}
            \gets
            s_q^{t,i-1}
            [
            f_i
            \leftarrow
            \widehat v_{q,i}^{t+1}
            ]\)
        \EndFor

        \State
        \(s_q^{t+1}
        \gets
        s_q^{t,4}\)

        \State
        \(\mathcal E_{\mathrm{hist}}
        \gets
\operatorname{Append}
\left(
\mathcal E_{\mathrm{hist}},
E_q^{t+1}
\right)\)

        \State
        \(d_q^{t+1}
        \gets
        \operatorname{Controller}
        (\nu_q^{t+1},t+1,T_{\max})\)

        \If{\(d_q^{t+1}=\textsc{Release}\)}
            \State
            \(E_q^\star
            \gets
            E_q^{t+1}\)
        \ElsIf{\(d_q^{t+1}=\textsc{Fallback}\)}
            \State
            \(E_q^\star
            \gets
            \operatorname{Merge}_{B}
            (\mathcal E_{\mathrm{hist}})\)
        \EndIf

        \State
        
         \(\operatorname{Persist}
        (\mathcal M,s_q^{t+1},d_q^{t+1})\)

        \If{\(d_q^{t+1}=\textsc{Revise}\)}
            \State
            \(c_q
            \gets
            \delta_q^{t+1}\)

            \State
            \(U_q^{t+1}
            \gets
            \operatorname{Resolve}
            (\mathcal M,q)\)
            \State \(s_q^{t+1}\gets s_q^{t+1}[U\leftarrow U_q^{t+1}]\)
        \Else
            \State
            \textbf{break}
        \EndIf
    \EndFor
\EndIf

\State
\(y_q
\gets
G_{\phi}
(q,E_q^\star)\)

\State
\Return \(y_q\)
\end{algorithmic}
\end{algorithm}
\section{Evaluation and Resource Accounting}
\label{sec:supp_evaluation}

\subsection{Workloads and Query Protocol}
\label{sec:supp_workloads}

We evaluate three LongBench QA tasks~\cite{bai-etal-2024-longbench}:
HotpotQA, 2WikiMQA, and MuSiQue. We additionally use the complete QASPER test split of 1,451
queries~\cite{dasigi-etal-2021-dataset} and a uniform sample of 2,000 queries
from the DocVQA validation split~\cite{mathew2021docvqa}.

All methods use the same query identifiers, source documents, and evaluation
order within each workload. The ordered query manifests record the workload, query identifier, source
identifier, and evaluation position. Section~\ref{sec:supp_implementation}
summarizes the shared execution environment and model assignments.

The source text supplied with each LongBench and QASPER query is treated as
its query associated source collection and processed with the evidence
segmentation procedure in Section~\ref{sec:supp_tam}. DocVQA uses the common
visual document preprocessing pipeline described in
Section~\ref{sec:supp_docvqa}.

For the main \textsc{StateRAG} evaluation, global memory \(M_g\) is empty at
the beginning of each workload. Eligible artifacts produced by earlier
queries remain available in a fixed query order within that workload.
Artifacts are not transferred across workloads. Gold answers, evaluation
labels, and final reader outputs are excluded from persistence. Task memory
and role private memory are cleared at each query boundary. In the matched
carrier control, both configurations additionally clear \(M_g\) at every
query boundary.

\begin{table*}[t]
\centering
\small
\setlength{\tabcolsep}{5pt}
\begin{tabular}{llllll}
\toprule
Workload & Split & Metrics & Macro weight & Error policy \\
\midrule
LongBench HotpotQA
& Evaluation 
& EM, F1, auxiliary Acc.
& \(1/3\)
& Zero, retained \\

LongBench 2WikiMQA
& Evaluation 
& EM, F1, auxiliary Acc.
& \(1/3\)
& Zero, retained \\

LongBench MuSiQue
& Evaluation 
& EM, F1, auxiliary Acc.
& \(1/3\)
& Zero, retained \\

QASPER
& Test 
& EM, F1, Acc.
& Not applicable
& Zero, retained \\

DocVQA
& Validation 
& ANLS, Acc.
& Not applicable
& Zero, retained \\
\bottomrule
\end{tabular}
\caption{Workloads and evaluation measures.}
\label{tab:supp_workloads}
\end{table*}

Incomplete executions and empty predictions receive zero for every applicable
quality metric and remain in the denominator. The auxiliary LongBench
accuracy measure is used only in the component and carrier analyses.

\subsection{Metric Definitions}
\label{sec:supp_metrics}

Let \(\widehat y_q\) denote the prediction for query \(q\), and let
\(\mathcal G_q\) be its set of reference answers. Answer normalization
lowercases text, removes punctuation and the English articles
\emph{a}, \emph{an}, and \emph{the}, and collapses consecutive whitespace.
Let \(\operatorname{norm}(x)\) denote the resulting string and
\(\operatorname{tok}(x)\) its whitespace separated token multiset.

Exact match against reference \(g\) is

\begin{equation}
\operatorname{EM}(\widehat y_q,g)
=
\mathbf{1}
\left[
\operatorname{norm}(\widehat y_q)
=
\operatorname{norm}(g)
\right].
\label{eq:supp_em}
\end{equation}

For token level F1, let \(o\) be the size of the multiset intersection between
\(\operatorname{tok}(\widehat y_q)\) and \(\operatorname{tok}(g)\). Precision,
recall, and F1 are

\begin{equation}
P=\frac{o}{|\operatorname{tok}(\widehat y_q)|},
\qquad
R=\frac{o}{|\operatorname{tok}(g)|},
\qquad
\operatorname{F1}
=
\frac{2PR}{P+R}.
\label{eq:supp_f1}
\end{equation}

F1 is zero when there is no token overlap. Accuracy uses normalized answer
containment:

\begin{equation}
\operatorname{Acc}(\widehat y_q,g)
=
\mathbf{1}
\left[
\begin{array}{c}
\operatorname{norm}(\widehat y_q)
\text{ is a substring of }
\operatorname{norm}(g)
\\
\text{or}
\\
\operatorname{norm}(g)
\text{ is a substring of }
\operatorname{norm}(\widehat y_q)
\end{array}
\right].
\label{eq:supp_accuracy}
\end{equation}

When a query has multiple reference answers, the query level score is the
maximum reference level score:

\begin{equation}
m_q
=
\max_{g\in\mathcal G_q}
m(\widehat y_q,g),
\qquad
m\in\{\operatorname{EM},\operatorname{F1},\operatorname{Acc}\}.
\label{eq:supp_multiple_gold}
\end{equation}

LongBench reports task level EM and F1. For a metric \(m\), its LongBench
macro value is the unweighted mean over the three tasks:

\begin{equation}
m_{\mathrm{LB}}
=
\frac{1}{3}
\left(
m_{\mathrm{HotpotQA}}
+
m_{\mathrm{2WikiMQA}}
+
m_{\mathrm{MuSiQue}}
\right).
\label{eq:supp_longbench_macro}
\end{equation}

The auxiliary LongBench accuracy measure is aggregated by the same rule.
QASPER reports EM, token level F1, and accuracy using the maximum over its
available references.

For DocVQA, let \(d_{\mathrm L}(x,y)\) be Levenshtein distance and define
normalized edit distance as

\begin{equation}
d_{\mathrm{norm}}(x,y)
=
\frac{
d_{\mathrm L}
\left(
\operatorname{norm}(x),
\operatorname{norm}(y)
\right)
}{
\max
\left(
|\operatorname{norm}(x)|,
|\operatorname{norm}(y)|
\right)
}.
\label{eq:supp_normalized_edit}
\end{equation}

The reference level ANLS score is

\begin{equation}
\operatorname{ANLS}(\widehat y_q,g)
=
\begin{cases}
1-d_{\mathrm{norm}}(\widehat y_q,g),
&
d_{\mathrm{norm}}(\widehat y_q,g)<0.5,
\\
0,
&
d_{\mathrm{norm}}(\widehat y_q,g)\geq0.5.
\end{cases}
\label{eq:supp_anls}
\end{equation}

DocVQA ANLS and accuracy are maximized over the available references.
Incomplete executions and empty predictions are assigned zero before
workload level aggregation.

\subsection{DocVQA Input Pipeline}
\label{sec:supp_docvqa}

For DocVQA, all methods use the same Qwen-VL-Plus front end to convert
document images into textual region level evidence. TAM organizes these
textual regions, and each Evidence node retains the generated text together
with its source page provenance. The same generated evidence is supplied to
all compared retrieval methods.

The final Qwen2.5-14B reader receives the query and selected textual evidence.
Raw document images are not passed to the final reader. TAM does not encode
bounding boxes or layout specific edges. The DocVQA experiment therefore
evaluates retrieval and state control over visual document evidence converted
into a common textual representation.

\subsection{Reader Equivalent Token Accounting}
\label{sec:supp_ret}

For a query \(q\), let \(\mathcal C_q\) contain every LLM call attributable
to that query. For call \(c\), let \(T_c\) be the total number of input and
output tokens, let \(m(c)\) be its executing model, and let \(N_{m(c)}\) and
\(N_{\mathrm R}\) denote the parameter counts of that model and the final
reader. Reader equivalent token usage is

\begin{equation}
\mathrm{RET}_q
=
\sum_{c\in\mathcal C_q}
\frac{N_{m(c)}}{N_{\mathrm R}}T_c .
\label{eq:supp_ret_general}
\end{equation}

The evaluated configuration uses Qwen2.5-14B as the final reader and
Qwen2.5-7B for the auxiliary and indexing calls of \textsc{StateRAG}. Under
this configuration, the reported accounting rule is

\begin{equation}
\mathrm{RET}_q
=
T_{q,\mathrm R}
+
\kappa
\left(
T_{q,\mathrm{aux}}+T_{q,\mathrm{idx}}
\right),
\qquad
\kappa=\frac{8}{14}.
\label{eq:supp_ret_reported}
\end{equation}

Here, \(T_{q,\mathrm R}\) contains the input and output tokens of the final
reader. The term \(T_{q,\mathrm{aux}}\) contains tokens from query time LLM
calls outside the final reader and index construction, including role
operations and Navigator path scoring. The term \(T_{q,\mathrm{idx}}\)
contains tokens from LLM calls used to construct retrieval structures
attributable to the query.

The nominal weight \(8/14\) conservatively upper bounds the parameter ratio
of the evaluated auxiliary and reader checkpoints. It provides a fixed
conversion for the reported 7B auxiliary and indexing calls. For methods that
use more than one model, each call is weighted by the parameter ratio of its
executing model. When every recorded call uses the reader checkpoint, all
tokens receive unit weight and RET equals the recorded total LLM token count.
An unavailable phase decomposition is not interpreted as zero use in that
phase.

For workload \(d\) with query set \(\mathcal Q_d\), mean RET is

\begin{equation}
\overline{\mathrm{RET}}_d
=
\frac{1}{|\mathcal Q_d|}
\sum_{q\in\mathcal Q_d}
\mathrm{RET}_q .
\label{eq:supp_mean_ret}
\end{equation}

All evaluated queries remain in the denominator. Tokens incurred before an
incomplete execution are retained. Query attributable index construction is
charged in full, while reusable corpus level construction is excluded from
per query RET. The reported values are computed from the execution logs
associated with the predictions in the main results table.

RET covers LLM token use under this accounting rule. Embedding computation,
graph traversal, CPU execution, network waiting time, and wall clock latency
are outside its scope.

\paragraph{Latency.}
For a completed query, \(L_q\) is measured from query submission to final
answer return. For an incomplete query, the interval ends at the recorded
termination or timeout. It includes query attributable indexing and online
execution, so

\begin{equation}
L_q
=
L_q^{\mathrm{idx}}
+
L_q^{\mathrm{online}}.
\label{eq:supp_latency}
\end{equation}

We report the arithmetic mean over the complete query manifest and retain the
elapsed time of incomplete executions.
\FloatBarrier
\section{Implementation and Baseline Alignment}
\label{sec:supp_implementation}

\subsection{Execution Environment}
\label{sec:supp_environment}

All experiments are executed on a local GPU server equipped with NVIDIA RTX
3090 GPUs. Preprocessing, retrieval, generation, and evaluation use Python
3.10 with PyTorch and the Hugging Face Transformers ecosystem.
Embedding based retrieval uses the sentence-transformers implementation of
\texttt{BAAI/bge-base-en-v1.5}. All methods are evaluated with the same
scoring implementation.

\begin{table}[t]
\centering
\small
\setlength{\tabcolsep}{4pt}
\begin{tabular}{@{}p{0.31\columnwidth}p{0.64\columnwidth}@{}}
\toprule
Component & Setting \\
\midrule
Hardware & Local server with NVIDIA RTX 3090 GPUs \\
Runtime & Python 3.10 \\
Model framework & PyTorch and Hugging Face Transformers \\
Embedding encoder & \texttt{BAAI/bge-base-en-v1.5} \\
Final reader & Qwen2.5-14B \\
Auxiliary model & Qwen2.5-7B \\
DocVQA front end & Qwen-VL-Plus \\
Decoding & Greedy with temperature \(0\) \\
\bottomrule
\end{tabular}
\caption{Shared implementation settings.}
\label{tab:supp_environment}
\end{table}

The Qwen2.5-14B model is used for final answer synthesis. Qwen2.5-7B is used
for auxiliary retrieval and control calls where required by the corresponding
method. For DocVQA, all methods share the Qwen-VL-Plus front end described in
Section~\ref{sec:supp_docvqa}. Greedy decoding with temperature \(0\) is used
throughout.

\subsection{StateRAG Model Interfaces}
\label{sec:supp_role_interfaces}

The Planner, Navigator, Retriever, and Verifier use fixed task instructions
and operate on the latest state available to their role. Table
\ref{tab:supp_role_contracts} summarizes the information presented to each
role and its required output. These contracts correspond to the typed fields
and validators defined in the main paper and in Section~\ref{sec:supp_lifecycle}.

\begin{table*}[t]
\centering
\small
\setlength{\tabcolsep}{6pt}
\begin{tabular}{p{0.13\textwidth}p{0.36\textwidth}p{0.41\textwidth}}
\toprule
Role & Input & Required output \\
\midrule
Planner &
Query, current state, and Verifier justification after
\textsc{Revise} &
A retrieval plan containing the current objective and retrieval targets \\

Navigator &
Query, committed plan, TAM, and admissible candidate traces &
One completed typed traversal trace ending at an Evidence node \\

Retriever &
Query, committed plan, and retrieval region determined by the committed path &
Evidence identifiers with source provenance, subject to the configured
evidence cap \\

Verifier &
Query and committed candidate evidence &
A \textsc{Pass} or \textsc{Fail} verdict with a brief justification \\

Final reader &
Query and the evidence selected by the terminal controller action &
One concise answer supported by the admitted evidence \\
\bottomrule
\end{tabular}
\caption{StateRAG role interfaces and output contracts.}
\label{tab:supp_role_contracts}
\end{table*}

Following \textsc{Revise}, the committed Verifier justification is included
in the next Planner input. The Navigator considers only transitions admitted
by the TAM type relation and proposes only completed traces. The Retriever
returns evidence from the region determined by the committed path. The
Verifier reads the resulting evidence and returns the categorical verdict
used by the controller.
\subsection{Baseline Implementations}
\label{sec:supp_baselines}

The comparison uses controlled implementations within a common evaluation
harness. Every method receives the same query manifest and source documents.
The Qwen2.5-14B final reader, reader prompt, maximum evidence token budget,
and scoring implementation are also shared. Each baseline retains the
indexing, traversal, reflection, or memory procedure that defines the cited
method. Its selected evidence is then passed through the common final reader
interface.

\begin{table*}[t]
\centering
\small
\setlength{\tabcolsep}{4pt}
\begin{tabular}{p{0.18\textwidth}p{0.43\textwidth}p{0.29\textwidth}}
\toprule
Method & Preserved retrieval or control procedure & Evidence passed to reader \\
\midrule
Vanilla RAG &
One similarity based passage retrieval pass &
Top ranked retrieved passages \\

DOSRAG~\cite{laitenberger-etal-2025-stronger} &
Passage retrieval followed by restoration to the original document order &
Selected passages in source order \\

ReAct~\cite{yao2023react} &
Interleaved reasoning, retrieval actions, and observations &
Evidence collected by the interaction trajectory \\

Self-RAG~\cite{asai2024selfrag} &
Reflection decisions controlling retrieval and passage assessment &
Evidence retained by the reflection procedure \\

RAPTOR~\cite{sarthi2024raptor} &
Recursive embedding, clustering, and summarization over a multilevel tree &
Nodes retrieved across abstraction levels \\

GraphRAG~\cite{edge2024graphrag} &
Entity graph construction, community detection, and community summaries &
Evidence retrieved from graph and community representations \\

MemoRAG~\cite{qian2025memorag} &
Corpus memory construction and memory generated clues that guide retrieval &
Evidence selected through clue guided retrieval \\

HippoRAG2~\cite{pmlr-v267-gutierrez25a} &
Passage and relation graph construction, recognition filtering, and
Personalized PageRank &
Evidence selected by the graph retrieval procedure \\
\bottomrule
\end{tabular}
\caption{Baseline procedures and common reader alignment.}
\label{tab:supp_baseline_alignment}
\end{table*}

For agentic baselines, the generated interaction trajectory remains internal
to the baseline procedure. Structured and memory based baselines retain their
native indexes and retrieval operations. The evaluation adapter converts only
the selected evidence into the shared reader input format.
\subsection{Prompt Templates}
\label{sec:supp_prompts}

The templates below reproduce the task instructions and required output fields
used in evaluation. Runtime serialization inserts the query, state, candidate,
and evidence content at the indicated positions. Differences limited to
whitespace are omitted. The auxiliary roles operate before final answer
synthesis and are not asked to answer the query.

\paragraph{TAM abstraction generator.}
The abstraction generator receives the target node type and the textual
representations of its child nodes.

\begin{quote}
\small
\raggedright
You generate a concise textual abstraction for a typed retrieval hierarchy.
Use only the information provided by the child nodes.

For a Relation node, describe the semantic relation connecting the supplied
evidence regions. For a Topic node, describe the broader subject shared by
the supplied Relation nodes. Preserve names, dates, entities, and relations
that may be needed for retrieval. Do not add unsupported information and do
not answer the user query.

\textbf{Node type:}
\(\{\text{node type}\}\)

\textbf{Child nodes:}
\(\{\text{child node text}\}\)

\textbf{Output:}

\textbf{ABSTRACTION:}
\end{quote}

\paragraph{Navigator and trace scorer.}
Candidate extensions are filtered by the TAM transition relation before they
are presented to the scorer. The scorer receives the query, committed plan,
and the ordered node sequence of each retained trace.

\begin{quote}
\small
\raggedright
You score candidate traversal traces in a typed retrieval hierarchy. Assess
how well the terminal abstraction of each trace supports the retrieval
objective expressed by the query and committed plan.

Assign one score between \(0\) and \(1\) to every supplied candidate. A higher
score indicates that continuing along the trace is more likely to reach
evidence needed for the query. Use only the supplied traces. Do not create
node identifiers, alter the node order, retrieve evidence, or answer the
query.

\textbf{Query:}
\(\{\text{query}\}\)

\textbf{Committed plan:}
\(\{\text{plan}\}\)

\textbf{Candidate traces:}
\(\{\text{candidate traces}\}\)

\textbf{Output:}

\textbf{TRACE\_ID:} \(\{\text{identifier}\}\),
\textbf{SCORE:} \(\{\text{score}\}\)
\end{quote}

The implementation retains the highest-scoring admissible traces under the
configured branch, beam, candidate, and depth limits. Only a completed trace
ending at an Evidence node can become the Navigator proposal.

\paragraph{Planner.}
The Planner receives the query and the latest retrieval state. Following
\textsc{Revise}, it also receives the committed Verifier justification.

\begin{quote}
\small
\raggedright
You are the Planner in a retrieval system. Define the current retrieval
objective and the information targets needed to answer the query. Use the
current state and any available reusable artifacts as context.

When revision context is present, update the plan to address the evidence
identified as missing by the Verifier. Do not select evidence, assess evidence
sufficiency, answer the query, or choose a controller action.

\textbf{Query:}
\(\{\text{query}\}\)

\textbf{Current retrieval state:}
\(\{\text{state}\}\)

\textbf{Available artifact identifiers:}
\(\{\text{artifacts}\}\)

\textbf{Revision context:}
\(\{\text{verifier justification or none}\}\)

\textbf{Output:}

\textbf{OBJECTIVE:}
\(\{\text{current retrieval objective}\}\)

\textbf{TARGETS:}
\(\{\text{ordered retrieval targets}\}\)
\end{quote}

The typed configuration validates this response as the proposal for \(p\).
The Planner does not update the path, evidence, verdict, or artifact fields.

\paragraph{Retriever.}
The Retriever receives only the candidate Evidence nodes associated with the
region selected by the committed traversal path.

\begin{quote}
\small
\raggedright
You are the Retriever in a retrieval system. Rank the supplied candidate
evidence by its relevance to the query and committed retrieval plan. Select
only evidence that contributes information needed to satisfy the current
objective.

Use only the supplied candidate evidence. Preserve the evidence identifiers
and source provenance. Do not introduce external information, assess final
evidence sufficiency, or answer the query. Select no more than the stated
evidence cap.

\textbf{Query:}
\(\{\text{query}\}\)

\textbf{Committed plan:}
\(\{\text{plan}\}\)

\textbf{Committed path:}
\(\{\text{typed path}\}\)

\textbf{Retrieval region:}
\(\{\text{region identifier}\}\)

\textbf{Candidate evidence:}
\(\{\text{evidence candidates with provenance}\}\)

\textbf{Evidence cap:}
\(\{\text{configured cap}\}\)

\textbf{Output:}

\textbf{SELECTED:}
\(\{\text{evidence identifiers in ranked order}\}\)
\end{quote}

The selected identifiers are resolved to evidence records carrying their
original provenance before the proposal is validated and committed to \(E\).

\paragraph{Verifier.}
The Verifier reads the query and the committed candidate evidence.

\begin{quote}
\small
\raggedright
You are the Verifier in a retrieval system. Determine whether the supplied
evidence is sufficient to answer the query.

Return \textsc{Pass} only when the evidence contains the information needed
to produce a supported answer. Return \textsc{Fail} when a required fact,
relation, comparison, or supporting step is missing. For \textsc{Fail},
identify the missing information that the next retrieval cycle should seek.

Judge evidence sufficiency only. Do not answer the query and do not select
\textsc{Release}, \textsc{Revise}, \textsc{Fallback}, or \textsc{Bypass}.

\textbf{Query:}
\(\{\text{query}\}\)

\textbf{Committed evidence:}
\(\{\text{evidence with provenance}\}\)

\textbf{Output:}

\textbf{VERDICT:}
\(\{\textsc{Pass} \text{ or } \textsc{Fail}\}\)

\textbf{JUSTIFICATION:}\\
\{brief evidence assessment or missing information\}
\end{quote}

The categorical verdict and its justification form the proposal for \(z\).
The controller selects the next action only after this proposal has been
validated and committed.

\paragraph{Final reader.}
All methods share the following final reader instruction:

\begin{quote}
\small
\raggedright
Answer the question using only the evidence below. Return the shortest answer
supported by the evidence and do not add an explanation. If the evidence is
incomplete, return the best supported answer from the available evidence.

\textbf{Question:}
\(\{\text{query}\}\)

\textbf{Evidence:}
\(\{\text{terminal evidence}\}\)

\textbf{Answer:}
\end{quote}

The final reader receives only the query and the evidence admitted by the
terminal controller action. Retrieval plans, traversal traces, Verifier
justifications, role trajectories, and memory contents are not added to the
reader prompt.

\paragraph{Carrier-specific rendering.}
The typed and free-form carrier configurations use the same role objectives,
inputs, model checkpoints, and task instructions. In the typed configuration,
the required output block for each role is interpreted as a proposal for its
designated field and is validated before commitment.

In the free-form configuration, the same task instruction is retained, while
the field-specific output wrapper is removed. Each role response is appended
as a natural-language record to the shared trajectory in execution order.
The controller does not reconstruct or validate the five-field schema.
Mechanical parsing is limited to retrieval tool arguments, selected evidence
identifiers, and the final \textsc{Pass} or \textsc{Fail} token. No repair
prompt, additional retry, or additional generation budget is provided.

\paragraph{DocVQA front end.}
The shared Qwen-VL-Plus front end uses the following instruction to convert a
document image into textual region evidence:

\begin{quote}
\small
\raggedright
Convert the supplied document image into faithful textual evidence for
document question answering. Preserve visible text, headings, labels, table
entries, and local associations needed to interpret the document. Organize
the output into concise textual regions in reading order.

Do not answer the user query and do not add information that is not visible
in the document. Associate each region with its page and region identifier.

\textbf{Document image:}
\(\{\text{document image}\}\)

\textbf{Output for each region:}

\textbf{PAGE:}
\(\{\text{page identifier}\}\)

\textbf{REGION\_ID:}
\(\{\text{region identifier}\}\)

\textbf{TEXT:}
\(\{\text{faithful textual content}\}\)
\end{quote}

The generated text and page provenance form the Evidence regions described in
Section~\ref{sec:supp_docvqa}. The controller, field validators,
compact-evidence predicate, and SMP access policy are deterministic procedures
and do not use additional LLM prompts.

\subsection{Parameter Selection and Resource Measurement}
\label{sec:supp_parameter_selection}

The StateRAG construction, navigation, retrieval, and lifecycle settings are
reported in Table~\ref{tab:supp_tam_settings} and Section~\ref{sec:supp_lifecycle}. Method specific
baseline parameters are selected on development data before evaluation. No
parameter is selected using the evaluation queries. Internal retrieval
settings follow the corresponding baseline procedure, while the maximum
evidence token budget admitted to the final reader remains common across
methods.

RET is computed from all recorded LLM calls using the accounting protocol in
Section~\ref{sec:supp_ret}. Query attributable index construction is charged
to the corresponding query. For a method that executes every LLM call with
the final reader checkpoint, every recorded token receives unit weight.
Incomplete executions retain the tokens consumed before termination.

End to end latency is measured on the execution environment reported in
Table~\ref{tab:supp_environment}. Timing begins at query submission and ends
when the final answer is returned. It includes query attributable index
construction and online execution. The arithmetic mean retains elapsed time
from incomplete executions and uses all evaluated queries as its denominator.
The workload order and memory reset conditions follow
Section~\ref{sec:supp_workloads}.
\FloatBarrier
\section{Component Ablations and Operational Profiles}
\label{sec:supp_components}

\subsection{Component Removal Settings}
\label{sec:supp_ablation_settings}

The Full configuration combines TAM, MARS, and SMP. The component study
removes one subsystem at a time while retaining the remaining retrieval
pipeline. All runs use the same evaluation queries, fixed query order, final
reader, scoring implementation, reader evidence budget, decoding settings,
and error policy. Checkpoints and prompts for components that remain active
are unchanged. Configured upper budgets are also retained where applicable,
although the number of executed calls may change when a subsystem is removed.

\begin{table*}[t]
\centering
\small
\setlength{\tabcolsep}{6pt}
\begin{tabular}{p{0.13\textwidth}p{0.40\textwidth}p{0.38\textwidth}}
\toprule
Variant & Removed scope & Retained execution \\
\midrule
w/o TAM &
TAM construction, typed path filtering, and typed navigation &
MARS state updates, SMP, the common reader interface, and answer scoring \\

w/o MARS &
Ordered role transitions, validation before commitment, and
Verifier conditioned revision &
TAM, SMP, the terminal reader interface, and answer scoring \\

w/o SMP &
The complete Shared Memory Pool, including \(M_g\), \(M_t\), \(M_a\), and
artifact resolution through \(U\) &
TAM, MARS, the live retrieval state, the common reader interface, and answer
scoring \\
\bottomrule
\end{tabular}
\caption{Scopes of the component removal variants.}
\label{tab:supp_ablation_definitions}
\end{table*}

The w/o SMP configuration removes the complete persistence subsystem. It is
separate from the matched carrier control in Section~\ref{sec:supp_carrier_control}, where both carriers
retain SMP and clear only \(M_g\) at each query boundary.

Table~\ref{tab:supp_ablation_differences} reports the Full minus removal
differences. All values are percentage points computed from the point
estimates reported in Table 2 of the main paper.

\begin{table}[!t]
\centering
\small
\setlength{\tabcolsep}{5pt}
\begin{tabular}{llrrr}
\toprule
Workload & Removal & \(\Delta\)EM & \(\Delta\)F1 & \(\Delta\)Acc. \\
\midrule
LongBench & w/o TAM  & 5.34 & 5.10 & 4.00 \\
          & w/o MARS & 8.84 & 9.49 & 7.50 \\
          & w/o SMP  & 6.00 & 6.29 & 4.30 \\
\midrule
QASPER   & w/o TAM  & 4.64 & 4.36 & 7.36 \\
         & w/o MARS & 4.56 & 5.68 & 4.91 \\
         & w/o SMP  & 3.54 & 5.25 & 6.54 \\
\bottomrule
\end{tabular}
\caption{Full minus removal point estimate differences.}
\label{tab:supp_ablation_differences}
\end{table}

MARS removal produces the largest LongBench decrease for all three metrics.
On QASPER, TAM removal produces the largest EM and accuracy decreases, while
MARS removal produces the largest F1 decrease. The largest observed decreases therefore vary across workloads and metrics.

\subsection{Operational Profiles}
\label{sec:supp_operational_profiles}

Figure~\ref{fig:supp_component_profiles} complements the removal comparisons
with three operational profiles over the 600 LongBench queries. Panel a
reports recorded mean LLM tokens attributed to index construction. The values
are 708 for StateRAG with TAM, 750 for GraphRAG, 29,144 for RAPTOR, and
151,851 for HippoRAG2.

Panel b compares the Full and w/o MARS LongBench point estimates. The
annotations report Full minus w/o MARS differences of 8.84 percentage points
for EM, 9.49 for F1, and 7.50 for accuracy.

Panel c reports access weighted global memory hit rates under the fixed query
order. The rates are 5.77 percent for HotpotQA, 17.45 percent for MuSiQue,
and 29.10 percent for 2WikiMQA. The reported LongBench aggregate is
17.44 percent.

\begin{figure*}[t]
    \centering
    \includegraphics[
    width=\textwidth,
]
{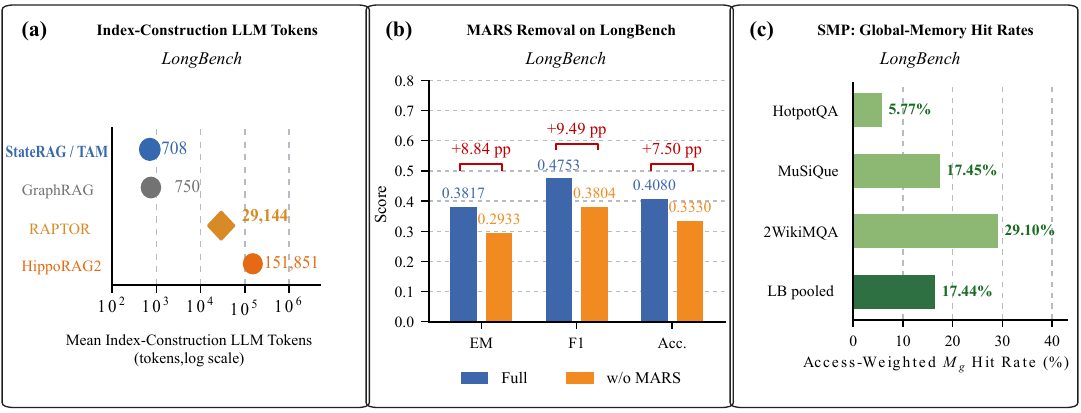}
    \caption{Descriptive component profiles on LongBench-600.}
    \label{fig:supp_component_profiles}
\end{figure*}

For a LongBench task \(d\), let \(A_d\) denote the number of permitted reads
from \(M_g\), and let \(H_d\) denote the number of those reads that return at
least one eligible artifact. The access weighted hit rate is

\begin{equation}
h_d
=
\frac{H_d}{A_d}.
\label{eq:supp_memory_hit_rate}
\end{equation}

Each permitted read contributes one access. Global memory is initialized
empty at the workload boundary and is retained under the fixed query order
within that workload. Figure~\ref{fig:supp_component_profiles} reports the
three task rates and the recorded LongBench aggregate.

The three panels connect TAM with index construction, MARS with state
transition, and SMP with artifact persistence. The component removal
comparisons report the corresponding outcome sensitivity under the evaluated
configurations.
\FloatBarrier
\section{Matched Carrier Control}
\label{sec:supp_carrier_control}

\subsection{Treatment Definition}
\label{sec:supp_carrier_treatment}
\begin{table*}[t]
\centering
\small
\setlength{\tabcolsep}{6pt}
\begin{tabular}{p{0.25\textwidth}p{0.33\textwidth}p{0.33\textwidth}}
\toprule
Dimension & Typed, role-owned carrier & Free-form shared carrier \\
\midrule
Carrier representation &
Five typed state fields &
One append-only shared trajectory \\

Recorded content &
Plan, typed path, evidence, verdict, and artifact identifiers &
Chronological Planner, Navigator, Retriever, and Verifier text \\

Write ownership &
Each role proposes values for its designated field &
All roles append to the shared trajectory \\

State update &
Validated proposal followed by controller commitment &
Direct textual append \\

Schema and type validation &
Enabled before commitment &
Disabled \\

API and output checks &
API success, nonempty output, and parsing required by each typed contract &
API success, nonempty output, and parsing only for tool arguments, evidence
identifiers, and the final \textsc{Pass} or \textsc{Fail} token \\

Role order &
Planner \(\rightarrow\) Navigator \(\rightarrow\) Retriever
\(\rightarrow\) Verifier &
The same order \\

TAM &
Same typed index, scorer, and navigation budgets &
The same configuration \\

SMP &
Retained &
Retained \\

Global memory \(M_g\) &
Cleared at every query boundary &
Cleared at every query boundary \\

Task memory \(M_t^q\) &
Retained within the query &
Retained within the query \\

Role private memory &
Retained within the query &
Retained within the query \\

Compact evidence rule &
Same rule and threshold &
The same rule and threshold \\

Controller actions &
\textsc{Bypass}, \textsc{Release}, \textsc{Revise}, and
\textsc{Fallback} &
The same actions \\

Budgets &
Same retrieval, evidence, context, and cycle budgets &
The same budgets \\

Final reader and scorer &
Same reader, prompt, decoding, and scoring implementation &
The same configuration \\
\bottomrule
\end{tabular}
\caption{Treatment definition for the matched carrier control.}
\label{tab:supp_carrier_treatment}
\end{table*}
The matched carrier control compares a typed, role-owned carrier with a
free-form shared carrier on the same 600 LongBench queries. Both
configurations use the same query identifiers, query order, source documents,
checkpoints, task instructions, decoding settings, TAM, SMP, retrieval
budgets, evidence budgets, controller cycle limit, reader prompt, and scoring
implementation.

The typed carrier stores the plan, typed path, evidence, verdict, and artifact
identifiers in five designated fields. The Planner, Navigator, Retriever, and
Verifier propose values for their assigned fields. The controller validates
each proposal before commitment.

The free-form carrier replaces these fields with one append-only textual
trajectory. Planner, Navigator, Retriever, and Verifier outputs are appended
in chronological order. The variant removes field ownership, schema
validation, type validation, and field-level commitment. The role order and
task instructions remain unchanged.

Mechanical parsing in the free-form configuration is limited to arguments
required by retrieval tools, selected evidence identifiers, and the final
\textsc{Pass} or \textsc{Fail} token. TAM continues to reject invalid node
identifiers and inadmissible transitions. These checks enforce tool validity
without reconstructing the five-field state contract.

Both configurations retain query-local artifact reuse through SMP. Clearing
\(M_g\) at each query boundary prevents earlier queries from influencing the
carrier comparison. A parse failure follows the shared error path. The
free-form variant receives no repair prompt, additional retry, or additional
generation budget. Both configurations use the same terminal evidence rules
and admit the final reader at most once.

The treatment therefore changes the state contract through three coordinated
properties. These are typed fields, designated write ownership, and validation
before commitment.

\subsection{Quality Results}
\label{sec:supp_carrier_quality}

Table~\ref{tab:supp_carrier_quality} reports the LongBench macro results. Each
macro value is the unweighted average over HotpotQA, 2WikiMQA, and MuSiQue.
The difference row is defined as Typed minus Free-form and is reported in
percentage points.

\begin{table}[!htbp]
\centering
\small
\setlength{\tabcolsep}{6pt}
\begin{tabular}{lrrr}
\toprule
Carrier & EM & F1 & Accuracy \\
\midrule
Typed, role-owned
& 0.3197 & 0.4081 & 0.3683 \\

Free-form shared
& 0.3067 & 0.3861 & 0.3383 \\

Typed minus Free-form
& \(+1.30\) & \(+2.20\) & \(+3.00\) \\
\bottomrule
\end{tabular}
\caption{LongBench macro results for the matched carrier control.}
\label{tab:supp_carrier_quality}
\end{table}

The typed, role-owned carrier records higher macro values for all three
metrics. The differences are 1.30 percentage points in EM, 2.20 in F1,
and 3.00 in accuracy.

\subsection{Token and RET Breakdown}
\label{sec:supp_carrier_resources}

Table~\ref{tab:supp_carrier_resources} reports the mean token components over
all 600 queries. Reader tokens include final reader input and output.
Auxiliary tokens include retrieval and control calls. Index tokens use the
same query attributable construction scope for both configurations.

\begin{table}[t]
\centering
\small
\setlength{\tabcolsep}{3pt}
\begin{tabular}{@{}lrrrr@{}}
\toprule
Carrier & Reader & Aux. & Index & RET \\
\midrule
Typed, role-owned
& 537.8 & 3,246.7 & 708.0 & 2,797.6 \\

Free-form shared
& 537.8 & 3,571.3 & 708.0 & 2,983.1 \\

Typed \(-\) Free-form
& 0.0 & \(-324.7\) & 0.0 & \(-185.5\) \\
\bottomrule
\end{tabular}
\caption{Carrier token and RET profiles.}
\label{tab:supp_carrier_resources}
\end{table}

RET is calculated using the model size weighting defined in
Section~\ref{sec:supp_ret}. Every evaluated query remains in the denominator,
and tokens produced before an incomplete execution are retained. Both
configurations use the same \(T_{\mathrm{idx}}\) definition and the same
weight \(\kappa=8/14\).

The typed carrier uses 324.7 fewer auxiliary tokens per query and lowers mean
RET by 185.5. Its mean RET is 6.2 percent lower than that of the free-form
carrier. Reader and index token means are unchanged under the reported
accounting.

\subsection{Execution Diagnostics}
\label{sec:supp_carrier_diagnostics}

Table~\ref{tab:supp_carrier_diagnostics} summarizes execution behavior from
the same runs used for the quality and resource results.

\begin{table}[!b]
\centering
\small
\setlength{\tabcolsep}{5pt}
\begin{tabular}{lrr}
\toprule
Diagnostic & Typed & Free-form \\
\midrule
Total queries & 600 & 600 \\
Parse failures & 0 & 4 \\
Incomplete executions & 5 & 8 \\
Context truncations & 1 & 4 \\
Reader admission violations & 0 & 0 \\
Cycles per query & 1.455 & 1.500 \\
Total LLM calls per query & 7.28 & 7.52 \\
Reader calls per query & 0.9917 & 0.9867 \\
Queries reaching the reader & 595/600 & 592/600 \\
\bottomrule
\end{tabular}
\caption{Execution diagnostics for the carrier control.}
\label{tab:supp_carrier_diagnostics}
\end{table}

A parse failure is recorded when a required value cannot be recovered under
the shared output checks. These cases follow the same incomplete execution
path used by the typed configuration. The free-form carrier receives no
additional parsing repair or retry budget.

Both configurations satisfy the reader admission invariant. No query invokes
the final reader more than once. The typed carrier records fewer parse
failures, incomplete executions, and context truncations, together with lower
mean cycle and call counts under the matched configuration.
\clearpage
\bibliography{references}

% Check whether the conference requires a reproducibility checklist to be included in the paper.
% If so, you can uncomment the following line and ajust the path to include it.
% \input{ReproducibilityChecklist.tex}

\end{document}
